# Supplementary material for: Understanding Contrastive Representation Learning through Alignment and Uniformity on the Hypersphere
Source: arXiv:2005.10242 source file (2022-08-15)
Supplement: Supplementary file 3 [file tbl_stl10.tex]

%auto-ignore
%!TEX root = ../../supplementary.tex

{
\scriptsize
\centering

\newcommand{\mroundprec}[1]{\round{#1}{2}\%}

\newcommand{\NA}{---}

% [inline block 0: 1 envs, 70192 chars -> data_tex | \begin{longtable}{r|c|c|c|c|c|c|c|c|c|c|c|c|} \caption{Experiment specifications for all $260$ \stl encoders. We report ...]

% }%
}
