# Supplementary material for: Understanding Contrastive Representation Learning through Alignment and Uniformity on the Hypersphere
Source: arXiv:2005.10242 source file (2022-08-15)
Supplement: Supplementary file 4 [file supplementary.tex]

%%%%%%%% ICML 2020 EXAMPLE LATEX SUBMISSION FILE %%%%%%%%%%%%%%%%%

\documentclass{article}

% Recommended, but optional, packages for figures and better typesetting:
\usepackage{microtype}
\usepackage{graphicx}
\usepackage{booktabs} % for professional tables

% hyperref makes hyperlinks in the resulting PDF.
% If your build breaks (sometimes temporarily if a hyperlink spans a page)
% please comment out the following usepackage line and replace
% \usepackage{icml2020} with \usepackage[nohyperref]{icml2020} above.
\usepackage{hyperref}

\usepackage[dvipsnames]{xcolor}
% Attempt to make hyperref and algorithmic work together better:

% Use the following line for the initial blind version submitted for review:
\usepackage{icml2020}
\usepackage{multirow}

% If accepted, instead use the following line for the camera-ready submission:
%\usepackage[accepted]{icml2020}

\hypersetup{colorlinks=true,linkcolor=blue,citecolor=blue}
\usepackage{amsmath}
\usepackage{amsfonts}
\usepackage[shortlabels]{enumitem}
\setlist[itemize]{leftmargin=20pt,topsep=-2pt,itemsep=0.15ex}
\setlist[enumerate]{leftmargin=20pt,topsep=-2pt,itemsep=0.15ex}
\usepackage{algorithm}
\usepackage{macros}
\usepackage{todonotes}
\usepackage[warn]{textcomp}
\usepackage{subcaption}
\usepackage[export]{adjustbox}
\usepackage{expl3}[2012-07-08]
\ExplSyntaxOn
\cs_new_eq:NN \fpeval \fp_eval:n
\ExplSyntaxOff

\setcounter{section}{0}

\usepackage{array,longtable,hhline}

\makeatletter

\newcommand\tblcelllabel[2]{#1\def\@currentlabel{#1}\label{#2}}

\def\LTHH@let#1{\futurelet\@tempb\LTHH@loop}

\def\LTHH@loop{%
  \ifx\@tempb`\edef\next##1{%
  \the\toks@\cr
  \noalign{\penalty-\@lowpenalty\vskip-\arrayrulewidth}%
  \omit
  \the\toks@\cr
  \noalign{\nobreak}%
  }\else\let\next\LTHH@let
  \ifx\@tempb:\if@tempswa\HH@add{\hskip\doublerulesep}\fi\@tempswatrue
      \HH@add{\@tempc\vline\@tempc}\else
  \ifx\@tempb~\@tempswafalse
           \if@firstamp\@firstampfalse\else\HH@add{&\omit}\fi
              \HH@add{\hfil}\else
  \ifx\@tempb-\@tempswafalse
           \if@firstamp\@firstampfalse\else\HH@add{&\omit}\fi
              \HH@add{\leaders\hrule\@height\arrayrulewidth\hfil}\else
  \errortoken
  \fi\fi\fi\fi
  \next}

\def\ltcline#1{%
  \noalign{\nobreak}%
  \omit\@firstamptrue\@tempswafalse
  \xdef\@tempc{\ifx\extrarowheight\HH@undef\hskip-.5\arrayrulewidth\fi}%
  \HH@xexpast\relax#1*0x\@@\toks@{}%
  \expandafter\LTHH@let\@tempa`%
}

\makeatother

% The \icmltitle you define below is probably too long as a header.
% Therefore, a short form for the running title is supplied here:
\icmltitlerunning{
    Understanding Contrastive Representation Learning through Geometry on the Hypersphere Supplementary Material
}

\begin{document}

\onecolumn
\icmltitle{
    % Uniformity is Key to Contrastive Representation Learning \\
    % Contrastive Representation Learning Optimizes Alignment and Uniformity on Hypersphere \\
    Understanding Contrastive Representation Learning through \\ Geometry on the Hypersphere Supplementary Material
    % Demystifying Contrastive Representation Learning: Alignment and Uniformity on Hypersphere \\
    % Alignment and Uniformity are All You Need \\
    % Fantastic Representation Transfer Measures and Where to Find Them? \\
}

% It is OKAY to include author information, even for blind
% submissions: the style file will automatically remove it for you
% unless you've provided the [accepted] option to the icml2020
% package.

% List of affiliations: The first argument should be a (short)
% identifier you will use later to specify author affiliations
% Academic affiliations should list Department, University, City, Region, Country
% Industry affiliations should list Company, City, Region, Country

% You can specify symbols, otherwise they are numbered in order.
% Ideally, you should not use this facility. Affiliations will be numbered
% in order of appearance and this is the preferred way.
\icmlsetsymbol{equal}{*}

\begin{icmlauthorlist}
\icmlauthor{Aeiau Zzzz}{equal,to}
\icmlauthor{Bauiu C.~Yyyy}{equal,to,goo}
\icmlauthor{Cieua Vvvvv}{goo}
\icmlauthor{Iaesut Saoeu}{ed}
\icmlauthor{Fiuea Rrrr}{to}
\icmlauthor{Tateu H.~Yasehe}{ed,to,goo}
\icmlauthor{Aaoeu Iasoh}{goo}
\icmlauthor{Buiui Eueu}{ed}
\icmlauthor{Aeuia Zzzz}{ed}
\icmlauthor{Bieea C.~Yyyy}{to,goo}
\icmlauthor{Teoau Xxxx}{ed}
\icmlauthor{Eee Pppp}{ed}
\end{icmlauthorlist}

\icmlaffiliation{to}{Department of Computation, University of Torontoland, Torontoland, Canada}
\icmlaffiliation{goo}{Googol ShallowMind, New London, Michigan, USA}
\icmlaffiliation{ed}{School of Computation, University of Edenborrow, Edenborrow, United Kingdom}

\icmlcorrespondingauthor{Cieua Vvvvv}{c.vvvvv@googol.com}
\icmlcorrespondingauthor{Eee Pppp}{ep@eden.co.uk}

% You may provide any keywords that you
% find helpful for describing your paper; these are used to populate
% the "keywords" metadata in the PDF but will not be shown in the document
\icmlkeywords{Machine Learning, ICML}

\vskip 0.3in

% this must go after the closing bracket ] following \twocolumn[ ...

% This command actually creates the footnote in the first column
% listing the affiliations and the copyright notice.
% The command takes one argument, which is text to display at the start of the footnote.
% The \icmlEqualContribution command is standard text for equal contribution.
% Remove it (just {}) if you do not need this facility.

\printAffiliationsAndNotice{}  % leave blank if no need to mention equal contribution
% \printAffiliationsAndNotice{\icmlEqualContribution} % otherwise use the standard text.

\input{text/supplementary-retry-first-principle}

\clearpage
\newpage
{\small
\bibliography{reference}
\bibliographystyle{icml2020}
}

\end{document}
